# Supplementary material for: DialogCC: An Automated Pipeline for Creating High-Quality Multi-Modal Dialogue Dataset
Source: arXiv:2212.04119 source file (2024-03-29)
Supplement: Supplementary file 1 [file dicussion.tex]

\section{Discussion} \label{supp_sec:discussion}

\paragraph{Dicussion about Societal Impact.}
As mentioned in the Limitation section, we need to carefully consider potential gender-bias issues for the fairness multi-modal dialogue search model. To mitigate this potential issue, we think of three strategies to remove the potential gender bias problem. 
First, we can adopt a fair sampling approach~\cite{wang2021gender} during training via contrastive learning, which considers gender distribution to be fair. 
Second, we can adopt post-hoc methods, such as Post-hoc Bias Mitigation (PBM)~\cite{kong2024mitigating} or Post-processing debiasing~\cite{wang2021gender}, in the dataset construction phase, particularly during alignment with CLIP. 
Lastly, we alternatively leverage fairness-focused vision-and-language pre-trained models, such as FairCLIP~\cite{wang2022fairclip}, as a function $f(\cdot)$. These strategies aim to minimize gender bias as effectively as possible.

Instead of generating social dialogues with GPT-4, we use verified dialogue datasets (\ie EmpatheticDialogues, Wizard-of-Wikipedia, DailyDialog, BlendedSkillTalk, PersonaChat) as seed dialogue to identify potential image-sharing moments in these seed dialogues. Therefore, we did not conduct a direct safety filtering process for the social dialogue datasets. However, since LLMs can generate harmful content, we can use tools like the Rewire API to remove potentially toxic content during the process of creating image descriptions with GPT-4. Additionally, GPT-4 could produce biased results due to name bias in the given dialogues~\cite{sheng2021revealing}, we randomly replaced all names in conversations with Top-10K names of US SSN applicants from 1990 to 2021. Following the previous studies~\cite{smith2021hi,kim2022soda}, this approach ensures a broad representation of names from diverse genders and ethnic backgrounds.
