# Supplementary material for: DialogCC: An Automated Pipeline for Creating High-Quality Multi-Modal Dialogue Dataset
Source: arXiv:2212.04119 source file (2024-03-29)
Supplement: Supplementary file 2 [file DialogCC_supp.pdf]

# DialogCC: Large-Scale Multi-Modal Dialogue Dataset

*Supplementary Material*  
[github.com/passing2961/DialogCC](https://github.com/passing2961/DialogCC)

## Contents

|                                                           |           |
|-----------------------------------------------------------|-----------|
| <b>A Details of Multi-Modal Dialogue Dataset Creation</b> | <b>2</b>  |
| A.1. Source Data Collection . . . . .                     | 2         |
| A.1.1 Source Dialogue Collection . . . . .                | 2         |
| A.1.2 Source Image-Caption Collection . . . . .           | 2         |
| A.2 Detailed Analysis of DialogCC . . . . .               | 2         |
| A.2.1 Scalability . . . . .                               | 2         |
| A.2.2 Diversity . . . . .                                 | 2         |
| A.2.3 Generalization . . . . .                            | 3         |
| A.3 Case Studies of DialogCC . . . . .                    | 5         |
| A.3.1 Comparison examples to MMDD . . . . .               | 5         |
| A.3.2 Examples of DialogCC . . . . .                      | 5         |
| <b>B Details of Experimental Settings</b>                 | <b>5</b>  |
| B.1. Baseline Models . . . . .                            | 5         |
| B.2. Implementation Details . . . . .                     | 5         |
| <b>C Extended Experiments</b>                             | <b>6</b>  |
| C.1. Text Retrieval . . . . .                             | 6         |
| C.2. Image Retrieval . . . . .                            | 6         |
| C.3. Robustness on Image Augmentation . . . . .           | 8         |
| C.4. Robustness on Text Augmentation . . . . .            | 8         |
| <b>References</b>                                         | <b>11</b> |

## A. Details of Multi-Modal Dialogue Dataset Creation

### A.1. Source Data Collection

This section describe how we collect the source dialogue and image-caption pairs used in creating DialogCC.

#### A.1.1 Source Dialogue Collection

We collect five text-only dialogue datasets (i.e., Wizard-of-Wikipedia [6], Persona-Chat [31], EmpatheticDialogues [20], DailyDialog [13], and BlendedSkillTalk [25]) through the ParlAI [16] framework, which provides many dialogue datasets online.

#### A.1.2 Source Image-Caption Collection

We download the Conceptual Captions 3M [24] (CC3M) dataset in here <sup>1</sup>. Since the CC3M dataset provides image URLs, we download images using `img2dataset` <sup>2</sup> library, which is a helpful library for quick downloading large-scale images based on URLs. We store downloaded images as a webdataset <sup>3</sup> format for efficiently extracting visual features by the CLIP [19] model. Note that because each image URL has the copyright, we only use opened URLs as source image-caption data when we create DialogCC.

### A.2. Detailed Analysis of DialogCC

In this section, we provide a detailed analysis of DialogCC in terms of the *scalability*, *diversity*, and *generalization*.

#### A.2.1 Scalability

Table A shows the full statistics of DialogCC compared to existing datasets MMDD [12] and PhotoChat [30]. As we aforementioned, DialogCC comprises of 92k unique dialogues in total, which is roughly  $3.7\times$  and  $7.7\times$  larger than MMDD and PhotoChat, respectively. Although the number of dialogue turn on average is shorter than existing datasets, the utterance length is longer than others, which indicates that our dataset contains more specific utterances that can increase the interestingness and engaigness [23]. For example, given the utterance “how are you?”, the response “I’m really good, because I’m going to paris today!” is more close to specific utterance than the response of “I’m good”. Thus, the multi-modal dialogue generative model trained on our dataset can generate more specific responses, making conversation more attractive.

<sup>1</sup><https://ai.google.com/research/ConceptualCaptions/download>

<sup>2</sup><https://github.com/rom1504/img2dataset>

<sup>3</sup><https://github.com/webdataset/webdataset>

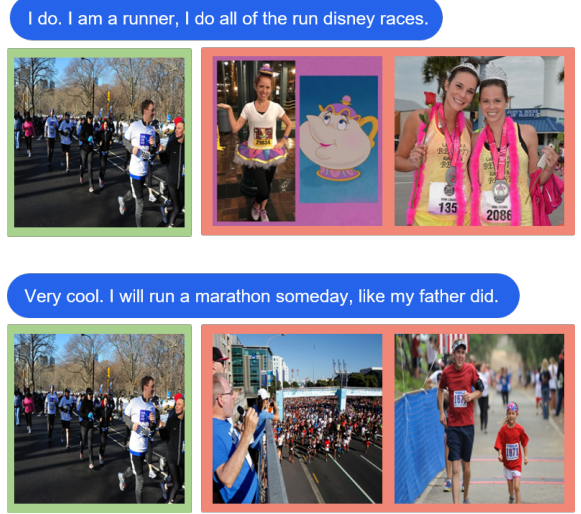

Figure A. **Problematic Examples in MMDD [12]**. Even if the two given utterances have different semantic meanings, MMDD matches the same image. Hence, training a multi-modal dialogue model with MMDD will likely memorize this **green** image rather than a deep understanding of input utterances. Images in the **green** box are from MMDD, images in the **red** box are from DialogCC, and the **blue** box is utterances.

Furthermore, we provide the detailed statistics of DialogCC according to the source dialogue datasets, as shown in Table B. Overall, the KnowledgeCC dataset includes the largest number of images per utterance and dialogue than other source dialogue datasets and the EmpathyCC has the smallest number. This result indicates that the CLIP similarity between image and utterance, which contains more object information (e.g., dog, bus, soccer), is relatively higher than the similarity between image and utterance related to the emotional situation.

#### A.2.2 Diversity

As shown in Section 3.2, DialogCC contains the largest number of unique hypernyms and unique words in both dialogues and image captions. In addition, we show that our dataset covers various conversational skills with balanced distribution, as illustrated in Figure 7 in our main paper. We furthermore compare the diversity of datasets in terms of the part-of-speech (POS) by using the pos tagger provided by the spaCy <sup>4</sup>. In total, compared to PhotoChat and MMDD, our dataset includes  $4.5\times$  and  $2.2\times$  more noun words;  $13.4\times$  and  $3.2\times$  more verb words;  $1.7\times$  and  $2.7\times$  more adjective words, which suggests that our dataset covers more variety of words.

<sup>4</sup><https://spacy.io/>

| Datasets        | Type  | # Unique Dialog | # Utter          | Avg. # Utter/Dialog | Avg. # Token/Utter | # Image          | # Unique Image | Avg. # Image/Dialog | Avg. # Image/Utter | Avg. # Utter/Image |
|-----------------|-------|-----------------|------------------|---------------------|--------------------|------------------|----------------|---------------------|--------------------|--------------------|
| MMDD [12]       | train | 21,411          | 519,728          | 13.01               | 11.97              | 39,956           | 12,272         | 3.32                | 1.87               | 3.26               |
|                 | valid | 2,400           | 32,708           | 13.62               | 11.87              | 2,401            | 334            | 1.13                | 1.0                | 7.19               |
|                 | test  | 2,672           | 36,315           | 13.59               | 11.85              | 2,673            | 682            | 1.13                | 1.0                | 3.92               |
|                 | total | 26,483          | 588,751          | 13.07               | 11.96              | 45,030           | 13,288         | 3.42                | 1.7                | 3.39               |
| PhotoChat [30]  | train | 10,286          | 130,459          | 12.68               | 6.33               | 10,286           | 8,889          | 1.0                 | 1.0                | 1.16               |
|                 | valid | 1,000           | 12,695           | 12.7                | 6.31               | 1,000            | 1,000          | 1.0                 | 1.0                | 1.0                |
|                 | test  | 1,000           | 12,841           | 12.84               | 6.29               | 1,000            | 1,000          | 1.0                 | 1.0                | 1.0                |
|                 | total | 12,286          | 155,995          | 12.7                | 6.33               | 12,286           | 10,889         | 1.0                 | 1.0                | 1.13               |
| DialogCC (ours) | train | 77,354          | 6,362,844        | 9.89                | 14.18              | 2,492,320        | 467,944        | 32.22               | 3.88               | 5.33               |
|                 | valid | 7,940           | 674,708          | 10.34               | 13.61              | 341,648          | 92,723         | 43.03               | 5.24               | 3.68               |
|                 | test  | 7,648           | 644,968          | 10.3                | 13.77              | 325,627          | 91,198         | 42.58               | 5.2                | 3.57               |
|                 | total | <b>92,942</b>   | <b>7,682,520</b> | <b>9.97</b>         | <b>14.09</b>       | <b>3,159,595</b> | <b>651,840</b> | <b>34.0</b>         | <b>4.1</b>         | <b>4.85</b>        |

Table A. **Full Statistics of Datasets.** Compared to existing datasets MMDD and PhotoChat, DialogCC includes the largest number of unique dialogues and images.

| Datasets    | Type  | # Unique Dialog | # Utter          | Avg. # Utter/Dialog | Avg. # Token/Utter | # Image          | # Unique Image | Avg. # Image/Dialog | Avg. # Image/Utter | Avg. # Utter/Image |
|-------------|-------|-----------------|------------------|---------------------|--------------------|------------------|----------------|---------------------|--------------------|--------------------|
| KnowledgeCC | train | 35,252          | 2,368,960        | 8.32                | 16.5               | 1,386,041        | 305,656        | 39.32               | 4.87               | 4.53               |
|             | valid | 1,952           | 131,556          | 8.33                | 16.53              | 132,398          | 42,352         | 67.83               | 8.39               | 3.13               |
|             | test  | 1,917           | 127,684          | 8.29                | 16.53              | 129,317          | 41,580         | 67.46               | 8.39               | 3.11               |
|             | total | <b>39,121</b>   | <b>2,628,200</b> | <b>8.32</b>         | <b>16.5</b>        | <b>1,647,756</b> | <b>389,574</b> | <b>42.12</b>        | <b>5.22</b>        | <b>4.23</b>        |
| PersonaCC   | train | 8,763           | 1,924,764        | 14.92               | 11.67              | 268,399          | 145,069        | 30.63               | 2.08               | 1.85               |
|             | valid | 1,000           | 244,500          | 15.67               | 11.92              | 54,333           | 31,169         | 54.33               | 3.48               | 1.74               |
|             | test  | 967             | 234,096          | 15.6                | 11.77              | 45,409           | 27,148         | 46.96               | 3.03               | 1.67               |
|             | total | <b>10,730</b>   | <b>2,403,360</b> | <b>15.06</b>        | <b>11.71</b>       | <b>368,141</b>   | <b>203,382</b> | <b>34.31</b>        | <b>2.31</b>        | <b>1.81</b>        |
| EmpathyCC   | train | 11,830          | 209,280          | 4.26                | 13.73              | 130,441          | 84,072         | 11.03               | 2.65               | 1.55               |
|             | valid | 2,151           | 38,280           | 4.27                | 14.62              | 27,739           | 19,597         | 12.9                | 3.1                | 1.42               |
|             | test  | 1,993           | 35,412           | 4.27                | 15.59              | 25,991           | 18,438         | 13.04               | 3.14               | 1.41               |
|             | total | <b>15,974</b>   | <b>282,972</b>   | <b>4.26</b>         | <b>14.08</b>       | <b>184,171</b>   | <b>122,104</b> | <b>11.53</b>        | <b>2.77</b>        | <b>1.51</b>        |
| DailyCC     | train | 16,934          | 1,240,428        | 9.69                | 14.11              | 550,047          | 161,406        | 32.48               | 4.3                | 3.41               |
|             | valid | 1,845           | 128,612          | 9.4                 | 13.67              | 68,686           | 24,760         | 37.23               | 5.02               | 2.77               |
|             | test  | 1,807           | 119,484          | 9.2                 | 14.14              | 72,060           | 28,214         | 39.88               | 5.55               | 2.55               |
|             | total | <b>20,586</b>   | <b>1,488,524</b> | <b>9.62</b>         | <b>14.07</b>       | <b>690,793</b>   | <b>214,375</b> | <b>33.56</b>        | <b>4.47</b>        | <b>3.22</b>        |
| BlendedCC   | train | 4,575           | 619,412          | 11.83               | 13.34              | 157,392          | 111,702        | 34.4                | 3.01               | 1.41               |
|             | valid | 992             | 131,760          | 11.75               | 13.48              | 58,492           | 37,133         | 58.96               | 5.22               | 1.58               |
|             | test  | 964             | 128,292          | 11.77               | 13.85              | 52,850           | 34,590         | 54.82               | 4.85               | 1.53               |
|             | total | <b>6,531</b>    | <b>879,464</b>   | <b>11.81</b>        | <b>13.44</b>       | <b>268,734</b>   | <b>183,418</b> | <b>41.15</b>        | <b>3.61</b>        | <b>1.47</b>        |

Table B. **Detailed Statistics of DialogCC.** We show the statistics on the results of matching each source dialogue dataset and CC3M. KnowledgeCC, PersonaCC, EmpathyCC, DailyCC, and BlendedCC denote the multi-modal dialogue dataset created from the Wizard-of-Wikipedia [6], Persona-Chat [31], EmpatheticDialogues [20], DailyDialog [13], and BlendedSkillTalk [25], respectively.

|                 | Dialog        |               |               | Image Caption |               |              | Total         |               |               |
|-----------------|---------------|---------------|---------------|---------------|---------------|--------------|---------------|---------------|---------------|
|                 | # noun        | # verb        | # adj         | # noun        | # verb        | # adj        | # noun        | # verb        | # adj         |
| MMDD            | 6,696         | 13,369        | 4,138         | 6,808         | 1,749         | 3,279        | 13,504        | 15,118        | 7,417         |
| PhotoChat       | 5,240         | 3,270         | 10,918        | 1,529         | 412           | 377          | 6,769         | 3,682         | 11,295        |
| DialogCC (Ours) | <b>15,976</b> | <b>35,522</b> | <b>11,652</b> | <b>14,822</b> | <b>13,921</b> | <b>8,567</b> | <b>30,798</b> | <b>49,443</b> | <b>20,219</b> |

Table C. **Part-of-Speech (POS) Comparison Results.** We count the number of the unique noun, verb, and adjective words in dialogues and image captions. # noun, # verb, and # adj denote the number of the unique noun word, the number of the unique verb words, and the number of the unique adjective words, respectively.

### A.2.3 Generalization

In real-life conversations, various images can be shared even with the same utterance, depending on who shares the

image. As shown in Table A, DialogCC contains larger images per utterance and dialogue than existing datasets, which indicates that our dataset can successfully reflect this phenomenon. For example, as shown in Figure B, our dataset includes various images with similar semantic meanings to the given utterance, which can induce the model to be more robust than a model trained with MMDD. In addition, MMDD contains the same images on two different utterances, as illustrated in Figure A. For example, in the first row of Figure A, the image in our dataset is relevant to the keyword “disney races” in the utterance, while MMDD cannot. This result will induce the degradation of generalization performance because the model trained on MMDD may prefer to memorize specific images rather than

There is a large canyon, vast grasslands, ancient forests and mountain lakes.

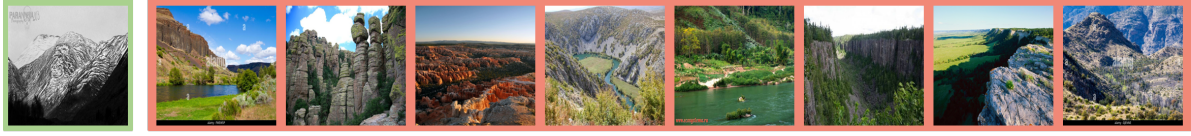

I am looking for a pair of shoes.

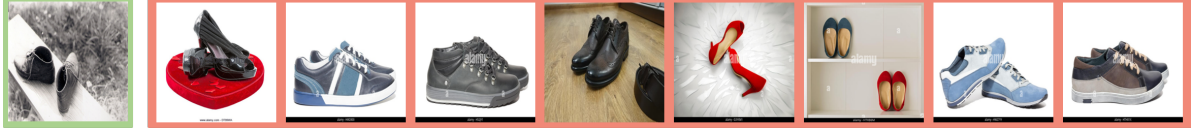

No, just two horses which I love.

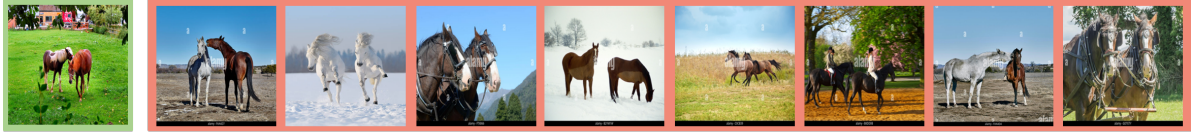

I am getting to go to my favorite cupcake bakery on monday!

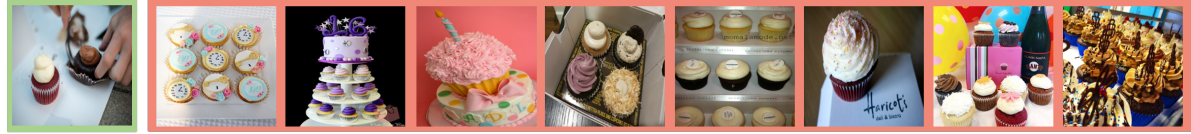

I used to be a corporate chef, but now I teach culinary school.

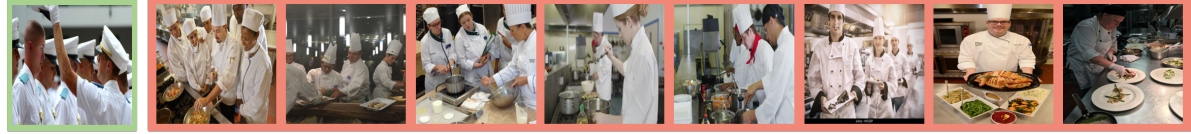

Soup does the body good, sweetie. It's what you need when you're under the weather.

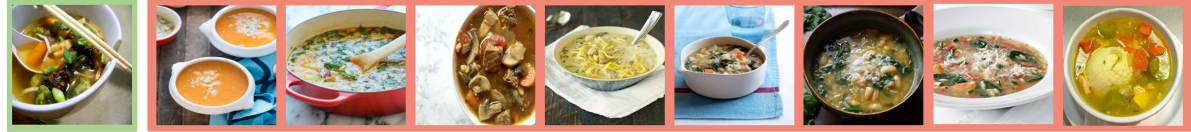

Rainy days are perfect for being lazy.

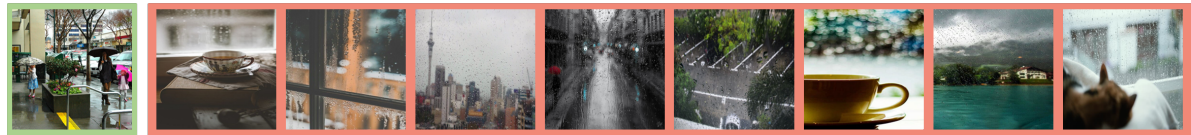

Well, maybe sneakers or rubber shoes.

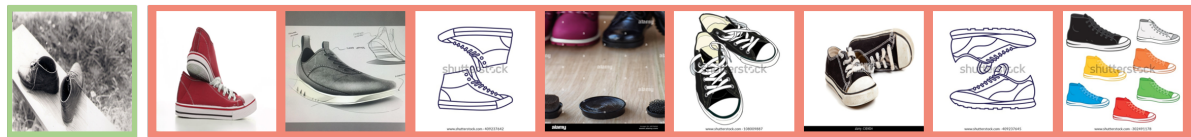

Figure B. **Comparison Examples of Relevant Images in MMDD [12] vs. DialogCC.** DialogCC contains various forms of images that are semantically similar to a given utterance. For example, in the top three rows, our dataset includes different kinds of “landscape”, “a pair of shoes”, and “two horses”. Besides, in the fifth row, unlike the MMDD, our dataset contains highly relevant images to the given utterance, which benefitted from the utterance-caption similarity. Images in the **green** box are from MMDD, images in the **red** box are from DialogCC, and the **blue** box is utterances.

understanding the dependency between image and utterance. We show that our dataset improves the generalization performance in Section 4.2.4, Section 4.2.5, Section C.3, and Section C.4.

### A.3. Case Studies of DialogCC

#### A.3.1 Comparison examples to MMDD

Unlike MMDD [12], we create DialogCC by using utterance-caption similarity as well as utterance-image similarity to improve the quality of DialogCC. To compare the different quality of multi-modal dialogue dataset, we present more comparison examples to MMDD in Figure B. In the last row of Figure B, our dataset includes more diverse images related to the “sneakers”, which are in the given utterance.

#### A.3.2 Examples of DialogCC

We present more examples of DialogCC in Figure G and Figure D. Both Figure G and Figure D show that DialogCC covers a variety of images, including various objects or scenes which are relevant to the given utterance, regardless of whether the conversation is short or long. For example, there are diverse images of graduation ceremonies, christmas, traffic jams, and hiking with a dog.

However, we sometimes found poor-quality examples of DialogCC, as illustrated in Figure F. On the second turn in the red box with a dotted line, the images are related to the given utterance that includes the word or phrase “pretty animal” or “arctic”. However, when we look at the previous utterance “Yes, I love huskys. They are a very pretty dog.”, we can easily recognize that these matched images are inappropriate to the given utterance considering the whole dialogue context. This is because when we calculate two similarities between utterance-caption and utterance-image by using CLIP model, we do not extract dialogue feature vectors or calculate the similarity by considering the whole dialogue context. Such a problem also exists in MMDD, which can be regarded as a typical problem of automatic methods [2, 12, 17] that can be utilized in creating several datasets. Nevertheless, recent studies have shown large-scale multi-modal pretraining models [1, 9, 11, 15, 19] have achieved enormous performance on various downstream tasks, which benefitted from the noisy large-scale image-caption datasets [3, 4, 21, 22, 26]. Therefore, this paper aims to create a large-scale multi-modal dialogue dataset, even if there is some noise, rather than creating a cleaned dataset.

## B. Details of Experimental Settings

### B.1. Baseline Models

As illustrated in Figure C, we present the architecture of baseline models, which is the text retrieval model [12] and

image retrieval model [30]. We provide a detailed description of baseline models below.

**Text Retrieval Model [12].** The text retrieval model consists of the dialogue, response, image, and multi-modal encoder. The dialogue encoder encodes the whole dialogue history into a fixed-size representation using the BERT [5] model. The response encoder converts the response into a fixed-size representation using the BERT model, the same BERT used in the dialogue encoder. They use the pooled vector from the BERT model to get the representations for dialogue history and response. When they encode the dialogue history, they use up to three turns just before the current turn by concatenating each turn with [SEP] special token. The image encoder is to extract image feature vectors using ResNeXt-101 [29]. After extracting text and image features, these features are fed into the fully-connected layer with the ReLU [18] activation function. They use the sum and attention modules to make a fused representation between the dialogue history and image. The sum module adds two vectors in an element-wise manner. They first concatenate the dialogue history vector and image feature vector for the attention module. They then pass the concatenated vector into the Transformer [27] to obtain contextualized multi-modal representation. Lastly, they calculate the dot product between the response feature vector and the multi-modal feature vector to get the loss.

**Image Retrieval Model [30].** The image retrieval model consists of a dialogue encoder, a caption encoder<sup>5</sup>, and an image encoder. The dialogue encoder and caption encoder leverage two different BERT models, which means the parameters of the two BERT models are not shared. They use the contextualized representation vector corresponding to the position of [CLS] for dialogue history and a caption. For the image encoder, they use ResNet-152 [8]. They concatenate two feature vectors for image and caption to obtain a meaningful multi-modal representation. They then pass the concatenated vector into the fully-connected layers with the ReLU function. They encode the dialogue history into a fixed-size representation and pass it to the fully-connected layers with the ReLU function. They calculate the cosine similarity by computing the dot product of L2 normalized features for dialogue history and multi-modal.

### B.2. Implementation Details

As we described the implementation details in our main paper, we explain additional implementation details for the extended experiments. Since our dataset is much larger than

<sup>5</sup>The original paper calls it a photo description encoder because PhotoChat contains the photo description per photo (image). In this paper, we call it the caption encoder.

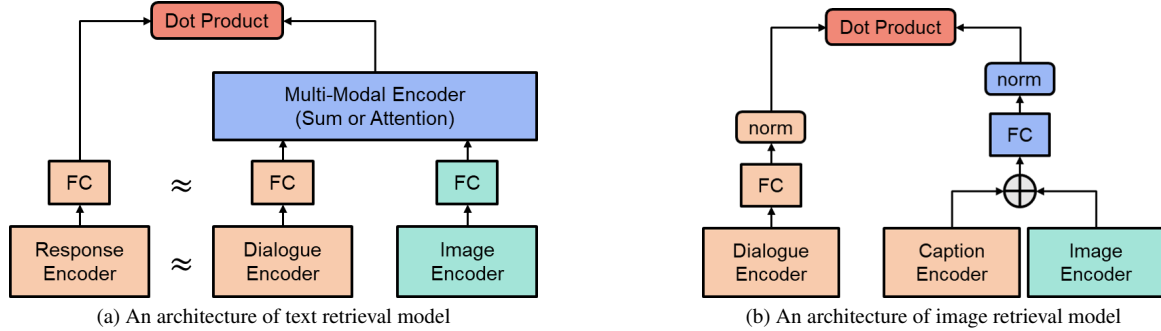

Figure C. **Architectures of Baseline Models.** We show the architecture of the text retrieval model [12] and image retrieval model [30], which are used in the experiment. We color the part corresponding to getting text representations as a light orange, the part corresponding to getting visual representation as a light green, and the part corresponding to getting a multi-modal representation as a light blue. The light red is the dot product.

the PhotoChat dataset, we use the cosine annealing schedule [14] with the same step size of 1,000. In all extended experiments, we train the models longer to achieve the best performance. We use the RandomResized cropping technique for image augmentation in both image retrieval and text retrieval experiments.

**Image Augmentation Techniques** For the experiment of robustness on image augmentation, we use the imgaug [10] library for image augmentation. We adopt eight image augmentation techniques, rotation, zoom-in, zoom-out, cutout, dropout, shearing, gaussian noise, and gaussian blur. We follow the same setting of each technique of the previous work [7].

**Text Augmentation Techniques** For the experiment of robustness on text augmentation, we use the synonym replacement techniques introduced in EDA [28].

## C. Extended Experiments

In this section, we show the extended experiments of the text retrieval and image retrieval models.

### C.1. Text Retrieval

Table D shows the text retrieval performance across all evaluation metrics, which is reported in our main paper. We train the model with more epochs to achieve improved performance. In addition, we conduct the ablation studies by applying different multi-modal encoders (i.e., sum and attention) and by changing model inputs, such as only providing the image or dialogue to the model, as shown in Table G. Even we further training, we observe a similar tendency that the model trained on our dataset improves the performance of MMDD. However, training the model with MMDD achieves considerably poor performance on our dataset. This result indicates that our dataset is more

challenging than MMDD due to the most significant number of images per utterance and dialogue. Moreover, such lack of diversity in MMDD induces the model to memorize seen images in the training process. The following paragraph explains the effect of different multi-modal encoders and model inputs.

**Effect of Multi-Modal Encoder.** In the model trained on MMDD, the sum module achieves better performance on two text retrieval tasks than the attention module, similar to the results reported in [12]. However, in the model trained on DialogCC, the attention module performs better on current turn prediction task. This result indicates that the attention module benefitted from the scalability and diversity of our dataset. In addition, the next turn prediction task is more challenging than the current turn prediction task due to the overall lower performance.

**Effect of Model Inputs.** To understand which modality is important in the text retrieval task, we conduct another experiment by giving different model inputs, such as only the dialogue history, only the image, or both the dialogue history and the image. Overall, using both modalities as input achieves the best performance. We also observe that considering dialogue history is important in the multi-modal dialogue retrieval tasks due to the lower performance of “Image Only”.

### C.2. Image Retrieval

Table E shows the image retrieval performance across all evaluation metrics, which is reported in Table 4 in our main paper. Since our dataset is larger and more diverse than PhotoChat, we need to train the image retrieval model with more epochs and vary the learning rate to achieve the best performance. Thus, we adopt the cosine annealing scheduler with a step size of 1,000. As shown in Table F, we

| Models↓        | Task →   | Current Turn Prediction |              |              |              |              |              | Next Turn Prediction |              |              |              |              |              |
|----------------|----------|-------------------------|--------------|--------------|--------------|--------------|--------------|----------------------|--------------|--------------|--------------|--------------|--------------|
|                | Eval →   | MMDD                    |              |              | DialogCC     |              |              | MMDD                 |              |              | DialogCC     |              |              |
|                | Train ↓  | R@1                     | R@5          | R@10         | R@1          | R@5          | R@10         | R@1                  | R@5          | R@10         | R@1          | R@5          | R@10         |
| BM25           | -        | 3.62                    | 7.91         | 10.46        | 0.72         | 4.48         | 8.05         | 3.72                 | 8.34         | 12.58        | 0.83         | 4.61         | 8.53         |
| Text Retrieval | MMDD     | 5.28                    | 16.18        | 23.34        | 2.65         | 7.73         | 11.29        | 2.93                 | 9.6          | 12.13        | 1.56         | 4.93         | 7.23         |
|                | DialogCC | <b>6.64</b>             | <b>21.57</b> | <b>30.16</b> | <b>10.17</b> | <b>28.74</b> | <b>39.17</b> | <b>4.31</b>          | <b>12.58</b> | <b>17.69</b> | <b>11.07</b> | <b>29.08</b> | <b>37.18</b> |

Table D. **Text Retrieval Performance.** We compare the performance of text retrieval model trained on DialogCC (when the maximum number of image is 10) and MMDD across all metrics.

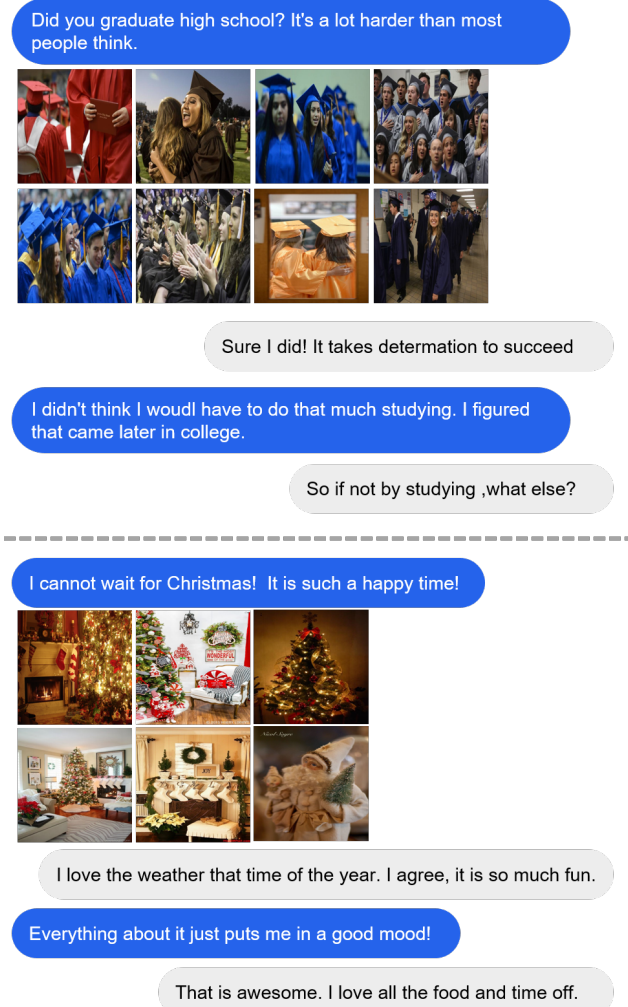

Figure D. **Case 1: Examples of DialogCC.** We present examples of DialogCC, and a gray dotted line separates each example. As illustrated in both examples, our dataset covers diverse images which are related to the utterance.

achieve the better performance than 7.58 (in Table E), which indicates that our dataset can make the model's training difficult due to the scalability and diversity. It will be helpful to improve the generalization performance.

| Models ↓        | Eval →<br>Train ↓ | PhotoChat   |              |              | DialogCC     |              |              |
|-----------------|-------------------|-------------|--------------|--------------|--------------|--------------|--------------|
|                 |                   | R@1         | R@5          | R@10         | R@1          | R@5          | R@10         |
| BM25            | -                 | 6.8         | 15.9         | 22.5         | 0.36         | 1.21         | 1.77         |
| Image Retrieval | PhotoChat         | 7.15        | <b>25.02</b> | <b>37.20</b> | 1.35         | 5.49         | 8.70         |
|                 | DialogCC          | <b>7.58</b> | 17.52        | 25.00        | <b>14.85</b> | <b>36.33</b> | <b>48.93</b> |

Table E. **Image Retrieval Performance.** We report the image retrieval performance on PhotoChat and DialogCC datasets, which is reported in Table 4 in our main paper.

| Eval →<br>Train ↓ | PhotoChat   |              |              | DialogCC    |              |              |
|-------------------|-------------|--------------|--------------|-------------|--------------|--------------|
|                   | R@1         | R@5          | R@10         | R@1         | R@5          | R@10         |
| PhotoChat         | 8.06        | <b>23.76</b> | <b>38.02</b> | 0.17        | 0.80         | 1.38         |
| DialogCC (1)      | 7.03        | 18.70        | 26.86        | 2.45        | 9.30         | 15.19        |
| DialogCC (5)      | 8.68        | 18.70        | 26.55        | 3.02        | 11.16        | 17.89        |
| DialogCC (10)     | 7.44        | 18.08        | 26.34        | 2.95        | 11.17        | 18.04        |
| DialogCC (15)     | <b>8.99</b> | 19.42        | 28.20        | <b>3.37</b> | <b>11.61</b> | <b>18.12</b> |
| DialogCC (20)     | 8.68        | 18.70        | 26.14        | 2.92        | 11.15        | 18.01        |
| DialogCC (30)     | 8.16        | 18.60        | 26.96        | 3.12        | 11.18        | 17.75        |

Table F. **Extended Image Retrieval Performance.** We report the image retrieval performance on PhotoChat and DialogCC dataset, where we train the image retrieval model with DialogCC by adopting the cosine annealing schedule. The number in parenthesis denotes the maximum number of images used in the training process.

However, the model trained on PhotoChat achieves better on R@5 and R@10. There are two possible reasons. The first reason is that the correlation between the training and test sets is larger in PhotoChat than in DialogCC. If the model trained on PhotoChat is well-generalized, it should have performed well in DialogCC, but it does not. On the other hand, training the model with our dataset shows high performance in both PhotoChat and DialogCC. The second reason is that the covered images in training, validation, and test set have similar domains in PhotoChat. PhotoChat only covers commonly shared objects, such as people, food, animal, and product. However, DialogCC is an open domain, which means that DialogCC covers many topics and conversational skills described in Section 3.2. This diversity would have decreased performance compared to the model trained on PhotoChat, which focuses on a specific domain. As shown in Figure E and Table F, the model trained on

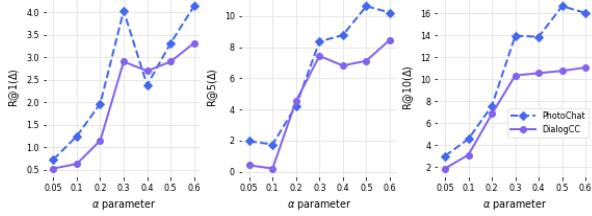

Figure E. **Performance Gap with Text Distortion.** We show the robustness performance of both models trained on our dataset or trained on PhotoChat by increasing the value of  $\alpha$ . The y-axis denotes the performance gap between the baseline score (without augmentation) and the score (with augmentation). The higher the value of the y-axis, the less robust the trained model is. This graph shows that the model trained on our dataset mostly achieves better robustness across all  $\alpha$  values.

DialogCC achieves better generalization performance than PhotoChat.

### C.3. Robustness on Image Augmentation

To explore whether our dataset can make a well-generalized model, we conduct a robust experiment by distorting image input. As shown in Table H, the model trained on our dataset shows a more robust performance with a lower reduction than the model trained on the MMDD dataset. This result implies that our dataset induces the model to be more robust to image distortion, which benefitted from the diversity of our dataset.

### C.4. Robustness on Text Augmentation

We evaluate the robustness of the model trained on our dataset by distorting input dialogue history. We replace randomly chosen words (except stopwords) with synonyms by adjusting the ratio of replacement  $\alpha$ . As shown in Figure E, the model trained on our dataset shows a more robust performance when the value of  $\alpha$  increases. This result indicates that while our dataset contains some noisy samples, our dataset makes the model more robust, which benefitted from the scalability and diversity of our dataset. Therefore, it is important to build a large-scale dataset to achieve improved generalization performance.

Yes, I love huskys. They are a very pretty dog.

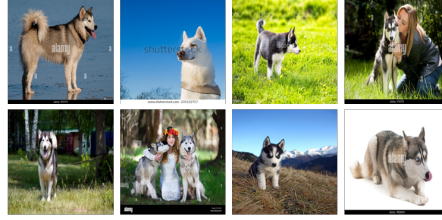

I agree - they are a very pretty animal. The word originated from the people "eskimo". Have you ever been to the arctic?

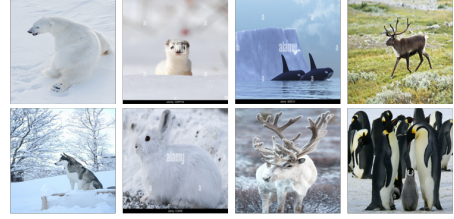

No I have not. Its too cold for me!

Great minds think alike - I don't want to go that far north either. It's crazy that not only have they evolved to live in such a cold climate, they have created their own languages as well!

I can't imagine having to live in an igloo!

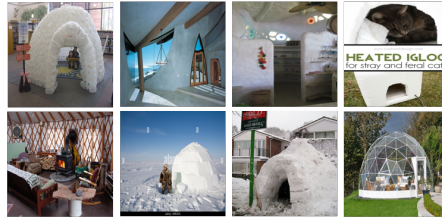

That would be so cold. I'd have to stay under a blanket all day! There is one igloo that I could stay inside and that is the software company. I'd love to have consistent employment with them!

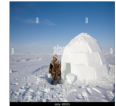

Consistent employment is very important. I miss my old job.

Yeah, that is key to supporting yourself. It's good to have an interview with an employer that you respect. Then you can assess if your talents with be of service.

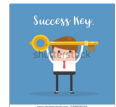

Figure F. **Case 3: Example of DialogCC that Unrelated to the Given Utterance.** In the red box with a dotted line, DialogCC contains diverse images that are relevant to the utterance. However, given the previous utterance, images should relate more to the "huskys" than many other animals, such as rabbits, polar bears, and penguins. Besides, it is more natural to share images related to "eskimo" or "arctic".

| MME↓      | Model Inputs↓    | Task→    | Current Turn Prediction |              |              |             |              |              | Next Turn Prediction |              |              |             |              |              |
|-----------|------------------|----------|-------------------------|--------------|--------------|-------------|--------------|--------------|----------------------|--------------|--------------|-------------|--------------|--------------|
|           |                  | Eval→    | MMDD                    |              |              | DialogCC    |              |              | ACL                  |              |              | DialogCC    |              |              |
|           |                  | Train↓   | R@1                     | R@5          | R@10         | R@1         | R@5          | R@10         | R@1                  | R@5          | R@10         | R@1         | R@5          | R@10         |
| Sum       | Image Only       | MMDD     | 5.37                    | 20.88        | 33.29        | 0.25        | 1.20         | 2.16         | 0.86                 | 3.12         | 5.48         | 0.09        | 0.37         | 0.65         |
|           |                  | DialogCC | 3.90                    | 15.67        | 24.90        | 1.01        | 4.27         | 6.94         | 1.67                 | 5.82         | 9.07         | 0.23        | 0.92         | 1.61         |
|           | Dialogue Only    | MMDD     | 8.55                    | 19.53        | 26.53        | 2.64        | 9.47         | 14.91        | 7.02                 | 15.79        | 21.22        | 3.52        | 10.45        | 14.96        |
|           |                  | DialogCC | 16.79                   | 35.92        | 45.55        | 5.22        | 20.28        | 29.47        | 16.26                | 32.65        | 40.52        | 7.02        | 21.94        | 30.15        |
|           | Dialogue + Image | MMDD     | 13.72                   | 35.68        | 49.48        | 0.95        | 3.95         | 6.70         | 6.80                 | 15.28        | 20.63        | 2.41        | 8.15         | 12.25        |
|           |                  | DialogCC | <b>15.16</b>            | <b>37.51</b> | <b>49.64</b> | <b>6.31</b> | <b>21.63</b> | <b>30.90</b> | <b>13.35</b>         | <b>30.81</b> | <b>39.62</b> | <b>6.64</b> | <b>21.22</b> | <b>29.51</b> |
| Attention | Image Only       | MMDD     | 5.01                    | 20.13        | 33.37        | 0.21        | 1.12         | 2.10         | 0.86                 | 3.47         | 5.73         | 0.09        | 0.40         | 0.72         |
|           |                  | DialogCC | 4.97                    | 16.99        | 26.93        | 1.08        | 2.94         | 6.74         | 1.37                 | 6.29         | 9.76         | 0.25        | 1.13         | 2.04         |
|           | Dialogue Only    | MMDD     | 8.83                    | 19.81        | 26.93        | 1.90        | 7.57         | 12.01        | 6.76                 | 15.32        | 20.92        | 3.28        | 10.45        | 15.55        |
|           |                  | DialogCC | 15.39                   | 33.17        | 42.64        | 5.40        | 20.03        | 29.80        | 16.09                | 34.28        | 42.88        | 7.17        | 22.76        | 31.34        |
|           | Dialogue + Image | MMDD     | 12.97                   | 33.13        | 45.55        | 0.92        | 3.57         | 6.23         | 4.66                 | 12.11        | 17.37        | 2.24        | 7.23         | 10.54        |
|           |                  | DialogCC | <b>19.49</b>            | <b>44.03</b> | <b>55.69</b> | <b>6.87</b> | <b>22.26</b> | <b>31.58</b> | <b>13.61</b>         | <b>30.51</b> | <b>38.55</b> | <b>5.04</b> | <b>15.76</b> | <b>22.71</b> |

Table G. **Extended Text Retrieval Performance.** We report the text retrieval performance on MMDD and DialogCC. MME denotes the multi-modal encoder.

| Train →        | MMDD         |               |               | DialogCC            |               |               |
|----------------|--------------|---------------|---------------|---------------------|---------------|---------------|
| Aug ↓          | R@1 (Δ)      | R@5 (Δ)       | R@10 (Δ)      | R@1 (Δ)             | R@5 (Δ)       | R@10 (Δ)      |
| Baseline       | 13.72        | 35.68         | 49.48         | 14.96               | 37.12         | 48.17         |
| Rotation       | 10.46 (3.26) | 30.27 (5.41)  | 41.89 (7.59)  | <b>13.25 (1.71)</b> | 32.62 (4.5)   | 43.16 (5.01)  |
| Zoom-In        | 7.52 (6.2)   | 22.43 (13.25) | 31.5 (17.98)  | <b>9.83 (5.13)</b>  | 25.18 (11.94) | 34.05 (14.12) |
| Zoom-Out       | 10.98 (2.74) | 31.07 (4.61)  | 42.32 (7.16)  | <b>13.6 (1.36)</b>  | 32.7 (4.42)   | 43.28 (4.89)  |
| Cutout         | 11.14 (2.58) | 31.11 (4.57)  | 43.56 (5.92)  | <b>12.85 (2.11)</b> | 32.54 (4.58)  | 43.44 (4.73)  |
| Dropout        | 9.03 (4.69)  | 25.54 (10.14) | 36.2 (13.28)  | <b>10.5 (4.46)</b>  | 27.73 (9.39)  | 37.79 (10.38) |
| Shearing       | 9.67 (4.05)  | 27.69 (7.99)  | 38.27 (11.21) | <b>12.25 (2.71)</b> | 31.19 (5.93)  | 41.25 (6.92)  |
| Gaussian noise | 10.46 (3.26) | 28.4 (7.28)   | 39.62 (9.86)  | <b>11.54 (3.42)</b> | 30.11 (7.01)  | 40.37 (7.8)   |
| Gaussian blur  | 10.78 (2.94) | 29.44 (6.24)  | 40.69 (8.79)  | <b>12.61 (2.35)</b> | 32.34 (4.78)  | 42.8 (5.37)   |

Table H. **Robustness Performance on Image Distortion.** We report the robustness performance when input images are distorted.

Hey, what do you do for a living?

Hello, I work in my mommas restaurant.

Oh nice, that is a cool job. What do you do for fun?

I read a lot, and go hiking with my dog.

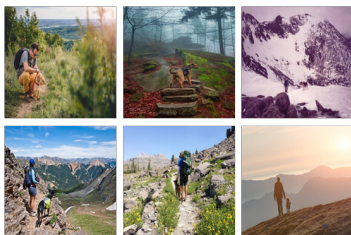

Those are both fun things to do.

I have seven siblings, one brother and six sisters. Are you an only child?

I am! Unless there are any surprise siblings that I do not know about.

Lucky you! What do you do for a living?

I work in a warehouse as a forklift operator!

That is not a bad job. I want to go to school next year.

What do you want to do at school?

Photography. I think I could make a decent living at it.

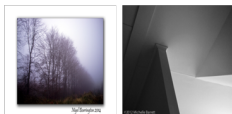

That would be an awesome job! Is photography a hobby of yours?

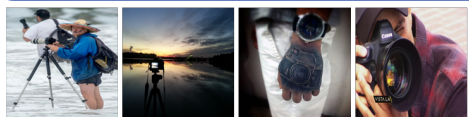

Yes it is, do you have any?

I got stuck in a traffic jam.

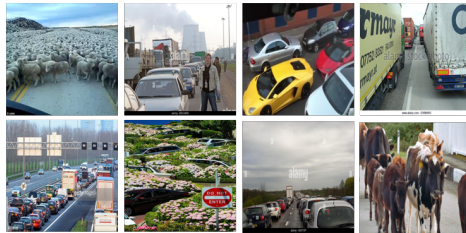

Hurry up , the show is about to start.

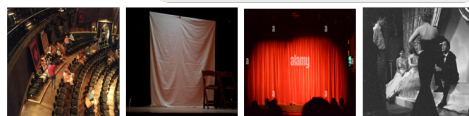

It looks like you're very interested in the circus.

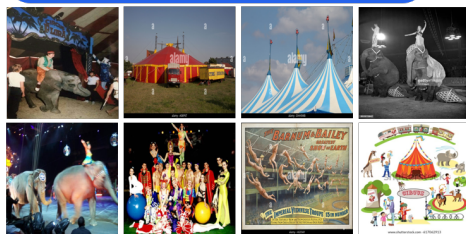

Yes , I love to see the animal show.

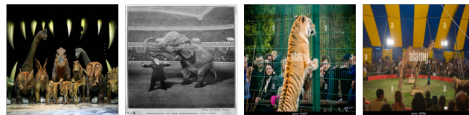

I have never seen those before, but since you're so excited it should be good.

I'm sure you'll love it.

Figure G. **Case 2: Examples of DialogCC.** We present examples of DialogCC. Both examples also treat various images relevant to the utterance. For example, in the left figure, our dataset includes images related to an utterance in which the motion is revealed “go hiking with my dog”.

## References

- [1] Jean-Baptiste Alayrac, Jeff Donahue, Pauline Luc, Antoine Miech, Iain Barr, Yana Hasson, Karel Lenc, Arthur Mensch, Katie Millican, Malcolm Reynolds, et al. Flamingo: a visual language model for few-shot learning. *arXiv preprint arXiv:2204.14198*, 2022. 5
- [2] Digbalay Bose, Rajat Hebbar, Krishna Somandepalli, Haoyang Zhang, Yin Cui, Kree Cole-McLaughlin, Huisheng Wang, and Shrikanth Narayanan. Movieclip: Visual scene recognition in movies. *arXiv preprint arXiv:2210.11065*, 2022. 5
- [3] Soravit Changpinyo, Piyush Sharma, Nan Ding, and Radu Soricut. Conceptual 12m: Pushing web-scale image-text pre-training to recognize long-tail visual concepts. In *Proceedings of the IEEE/CVF Conference on Computer Vision and Pattern Recognition*, pages 3558–3568, 2021. 5
- [4] Karan Desai, Gaurav Kaul, Zubin Aysola, and Justin Johnson. Redcaps: Web-curated image-text data created by the people, for the people. *arXiv preprint arXiv:2111.11431*, 2021. 5
- [5] Jacob Devlin, Ming-Wei Chang, Kenton Lee, and Kristina Toutanova. Bert: Pre-training of deep bidirectional transformers for language understanding. *arXiv preprint arXiv:1810.04805*, 2018. 5
- [6] Emily Dinan, Stephen Roller, Kurt Shuster, Angela Fan, Michael Auli, and Jason Weston. Wizard of wikipedia: Knowledge-powered conversational agents. *arXiv preprint arXiv:1811.01241*, 2018. 2, 3
- [7] Geonmo Gu, Byungsoo Ko, and Han-Gyu Kim. Proxy synthesis: Learning with synthetic classes for deep metric learning. In *Proceedings of the AAAI Conference on Artificial Intelligence*, volume 35, pages 1460–1468, 2021. 6
- [8] Kaiming He, Xiangyu Zhang, Shaoqing Ren, and Jian Sun. Deep residual learning for image recognition. In *Proceedings of the IEEE conference on computer vision and pattern recognition*, pages 770–778, 2016. 5
- [9] Chao Jia, Yinfei Yang, Ye Xia, Yi-Ting Chen, Zarana Parekh, Hieu Pham, Quoc Le, Yun-Hsuan Sung, Zhen Li, and Tom Duerig. Scaling up visual and vision-language representation learning with noisy text supervision. In *International Conference on Machine Learning*, pages 4904–4916. PMLR, 2021. 5
- [10] Alexander B. Jung, Kentaro Wada, Jon Crall, Satoshi Tanaka, Jake Graving, Christoph Reinders, Sarthak Yadav, Joy Banerjee, Gábor Vecsei, Adam Kraft, Zheng Rui, Jirka Borovec, Christian Vallentin, Semen Zhydenko, Kilian Pfeiffer, Ben Cook, Ismael Fernández, François-Michel De Rainville, Chi-Hung Weng, Abner Ayala-Acevedo, Raphael Meudec, Matias Laporte, et al. imgaug. <https://github.com/aleju/imgaug>, 2020. Online; accessed 01-Feb-2020. 6
- [11] Byungsoo Ko and Geonmo Gu. Large-scale bilingual language-image contrastive learning. *arXiv preprint arXiv:2203.14463*, 2022. 5
- [12] Nyoungwoo Lee, Suwon Shin, Jaegul Choo, Ho-Jin Choi, and Sung-Hyun Myaeng. Constructing multi-modal dialogue dataset by replacing text with semantically relevant images. *arXiv preprint arXiv:2107.08685*, 2021. 2, 3, 4, 5, 6
- [13] Yanran Li, Hui Su, Xiaoyu Shen, Wenjie Li, Ziqiang Cao, and Shuzi Niu. Daildialog: A manually labelled multi-turn dialogue dataset. *arXiv preprint arXiv:1710.03957*, 2017. 2, 3
- [14] Ilya Loshchilov and Frank Hutter. Sgdr: Stochastic gradient descent with warm restarts. *arXiv preprint arXiv:1608.03983*, 2016. 6
- [15] Jiasen Lu, Dhruv Batra, Devi Parikh, and Stefan Lee. Vilbert: Pretraining task-agnostic visiolinguistic representations for vision-and-language tasks. *Advances in neural information processing systems*, 32, 2019. 5
- [16] A. H. Miller, W. Feng, A. Fisch, J. Lu, D. Batra, A. Bordes, D. Parikh, and J. Weston. Parlai: A dialog research software platform. *arXiv preprint arXiv:1705.06476*, 2017. 2
- [17] Arsha Nagrani, Paul Hongsuck Seo, Bryan Seybold, Anja Hauth, Santiago Manen, Chen Sun, and Cordelia Schmid. Learning audio-video modalities from image captions. *arXiv preprint arXiv:2204.00679*, 2022. 5
- [18] Vinod Nair and Geoffrey E Hinton. Rectified linear units improve restricted boltzmann machines. In *ICML*, 2010. 5
- [19] Alec Radford, Jong Wook Kim, Chris Hallacy, Aditya Ramesh, Gabriel Goh, Sandhini Agarwal, Girish Sastry, Amanda Askell, Pamela Mishkin, Jack Clark, et al. Learning transferable visual models from natural language supervision. In *International Conference on Machine Learning*, pages 8748–8763. PMLR, 2021. 2, 5
- [20] Hannah Rashkin, Eric Michael Smith, Margaret Li, and Y-Lan Boureau. Towards empathetic open-domain conversation models: A new benchmark and dataset. *arXiv preprint arXiv:1811.00207*, 2018. 2, 3
- [21] Christoph Schuhmann, Romain Beaumont, Richard Vencu, Cade Gordon, Ross Wightman, Mehdi Cherti, Theo Coombes, Aarush Katta, Clayton Mullis, Mitchell Wortsman, et al. Laion-5b: An open large-scale dataset for training next generation image-text models. *arXiv preprint arXiv:2210.08402*, 2022. 5
- [22] Christoph Schuhmann, Richard Vencu, Romain Beaumont, Robert Kaczmarczyk, Clayton Mullis, Aarush Katta, Theo Coombes, Jenia Jitsev, and Aran Komatsuzaki. Laion-400m: Open dataset of clip-filtered 400 million image-text pairs. *arXiv preprint arXiv:2111.02114*, 2021. 5
- [23] Abigail See, Stephen Roller, Douwe Kiela, and Jason Weston. What makes a good conversation? how controllable attributes affect human judgments. *arXiv preprint arXiv:1902.08654*, 2019. 2
- [24] Piyush Sharma, Nan Ding, Sebastian Goodman, and Radu Soricut. Conceptual captions: A cleaned, hypernymed, image alt-text dataset for automatic image captioning. In *Proceedings of the 56th Annual Meeting of the Association for Computational Linguistics (Volume 1: Long Papers)*, pages 2556–2565, 2018. 2
- [25] Eric Michael Smith, Mary Williamson, Kurt Shuster, Jason Weston, and Y-Lan Boureau. Can you put it all together: Evaluating conversational agents’ ability to blend skills. *arXiv preprint arXiv:2004.08449*, 2020. 2, 3

- [26] Krishna Srinivasan, Karthik Raman, Jiecao Chen, Michael Bendersky, and Marc Najork. Wit: Wikipedia-based image text dataset for multimodal multilingual machine learning. In *Proceedings of the 44th International ACM SIGIR Conference on Research and Development in Information Retrieval*, pages 2443–2449, 2021. 5
- [27] Ashish Vaswani, Noam Shazeer, Niki Parmar, Jakob Uszkoreit, Llion Jones, Aidan N Gomez, Łukasz Kaiser, and Illia Polosukhin. Attention is all you need. *Advances in neural information processing systems*, 30, 2017. 5
- [28] Jason Wei and Kai Zou. Eda: Easy data augmentation techniques for boosting performance on text classification tasks. *arXiv preprint arXiv:1901.11196*, 2019. 6
- [29] Saining Xie, Ross Girshick, Piotr Dollár, Zhuowen Tu, and Kaiming He. Aggregated residual transformations for deep neural networks. In *Proceedings of the IEEE conference on computer vision and pattern recognition*, pages 1492–1500, 2017. 5
- [30] Xiaoxue Zang, Lijuan Liu, Maria Wang, Yang Song, Hao Zhang, and Jindong Chen. Photochat: A human-human dialogue dataset with photo sharing behavior for joint image-text modeling. *arXiv preprint arXiv:2108.01453*, 2021. 2, 3, 5, 6
- [31] Saizheng Zhang, Emily Dinan, Jack Urbanek, Arthur Szlam, Douwe Kiela, and Jason Weston. Personalizing dialogue agents: I have a dog, do you have pets too? *arXiv preprint arXiv:1801.07243*, 2018. 2, 3
